# Supplementary material for: Honeybee-like collective decision making in a kilobot swarm
Source: arXiv:2310.15592 ancillary file (2024-09-02)
Supplement: Supplementary file 1 [file suppMat.pdf]

# Supplementary Material for:
# 'Honeybee-like collective decision making in a kilobot swarm'

David March-Pons,[1,*] Julia Múgica,[1] Ezequiel E. Ferrero,[2,3] and M. Carmen Miguel[2,3]

[1] *Departament de Física, Universitat Politècnica de Catalunya, Campus Nord B4, 08034 Barcelona, Spain*
[2] *Departament de Física de la Matèria Condensada, Universitat de Barcelona, Martí i Franquès 1, 08028 Barcelona, Spain.*
[3] *Institute of Complex Systems (UBICS), Universitat de Barcelona, Barcelona, Spain*

[*] david.march@upc.edu

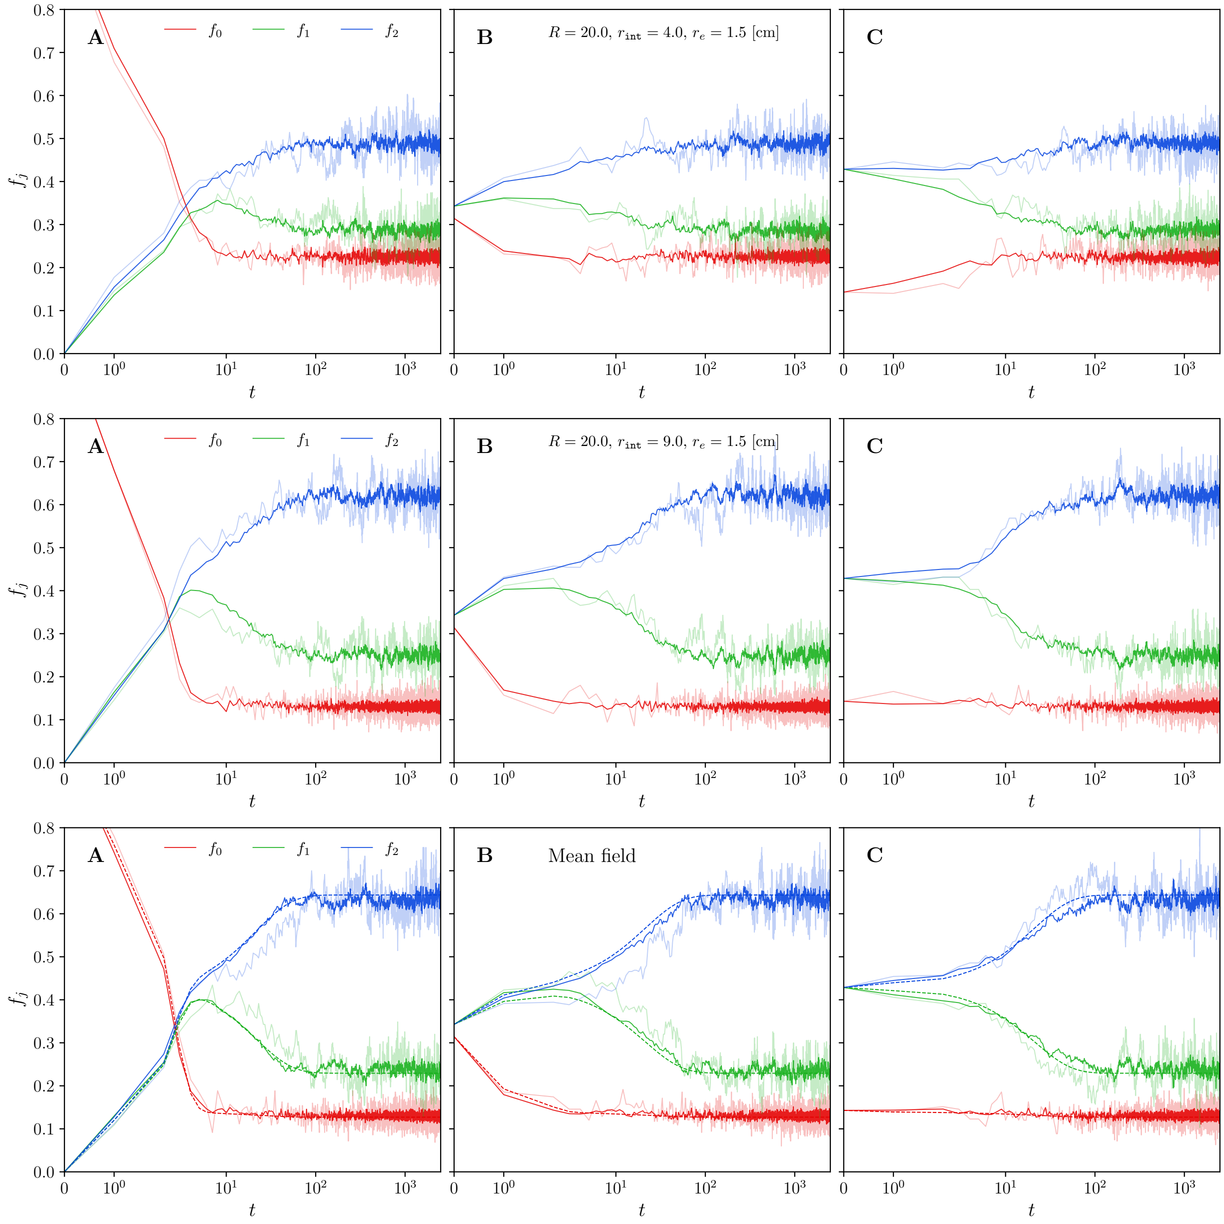


FIG. 1. Effect of initial conditions on the model dynamics on quenched networks configurations (top and middle rows) and mean field simulations (bottom row). Quenched parameters are arena radius $R = 20$ cm, agent body size $r_e = 1.5$ cm, interaction range $r_{\mathtt{int}} = 4.0$ cm (top row) and $r_{\mathtt{int}} = 9.0$ cm (middle row). Simulation parameters are: $N = 35$, $\pi_1 = \pi_2 = 0.3$, $q_1 = 7$, $q_2 = 10$, $\lambda = 0.6$. Columns correspond to the different initial conditions, **A**: $f_\alpha(t = 0) = (1, 0, 0)$. **B**: $f_\alpha(t = 0) \simeq (1/3, 1/3, 1/3)$. **C**: $f_\alpha(t = 0) = (0.13, 0.43, 0.43)$. Solid lines (semitransparent) are averages over 100 (10) realizations.

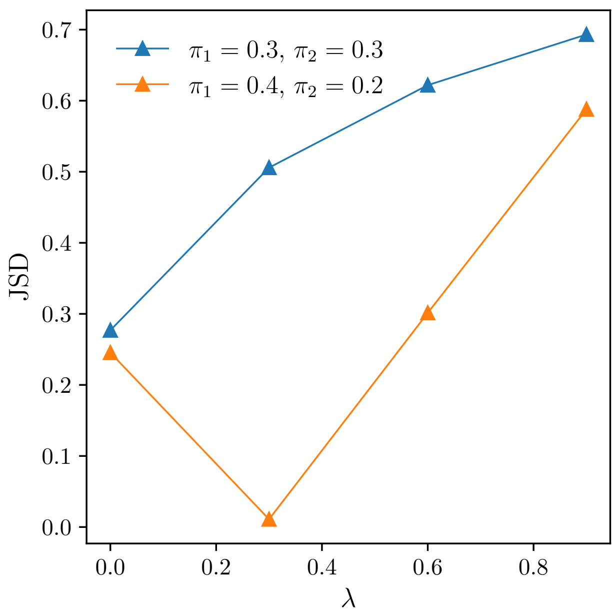


FIG. 2. Jensen Shannon Divergence (JSD) of the probability distributions from the population fractions $f_1$ and $f_2$ obtained from the kilobot experiments, with two different conditions: symmetric (asymmetric) discovery probabilities $\pi_1 = \pi_2 = 0.3$, blue line ($\pi_1 = 0.4$, $\pi_2 = 0.2$, orange line). This distributions are depicted in Figure 2, in the main paper.

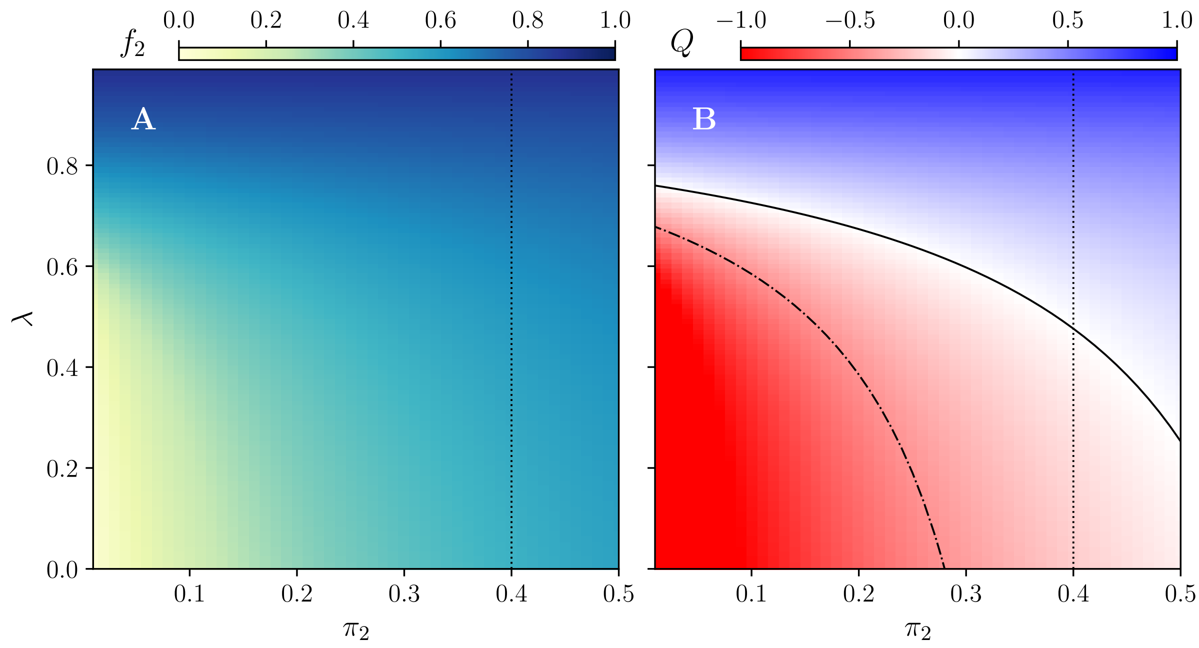


FIG. 3. Mean field analytical values of $f_2$ (**A**) and $Q$ (**B**) in the $(\pi_2, \lambda)$-parameter space, for the asymmetric scenario with $\pi_1 = 0.4$. The vertical dotted line indicates the constant value of $\pi_1$, the continuous line indicates the consensus crossover line and the dashed-dotted line indicates the simple majority consensus crossover line.

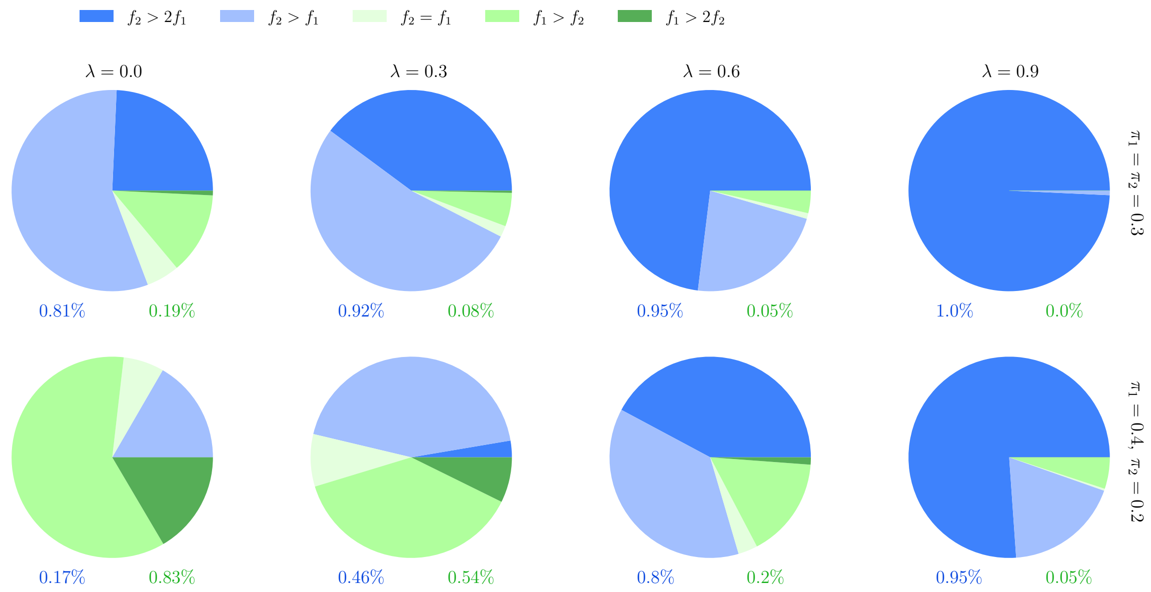


FIG. 4. Probability for the consensus outcomes in kilobot experiments ($N = 35$): optimal choice ($f_2 > 2f_1$, dark blue or $f_2 > f_1$, light blue) or sub-optimal choice ($f_1 > 2f_2$, dark green or $f_1 > f_2$, light green or $f_1 = f_2$, pale green). **Top row**: symmetric discovery case, $\pi_1 = \pi_2 = 0.3$. **Bottom row**: asymmetric discovery case, $\pi_1 = 0.4,\ \pi_2 = 0.2$. Columns indicate different choices of the interdependence, from left to right: $\lambda = 0.0,\ 0.3,\ 0.6,\ 0.9$. The percentage of times an optimal choice ($f_2$ wins) or sub-optimal choice (draw or $f_1$ wins) is indicated under each chart, on the left (blue-colored) and right (green-colored), respectively.

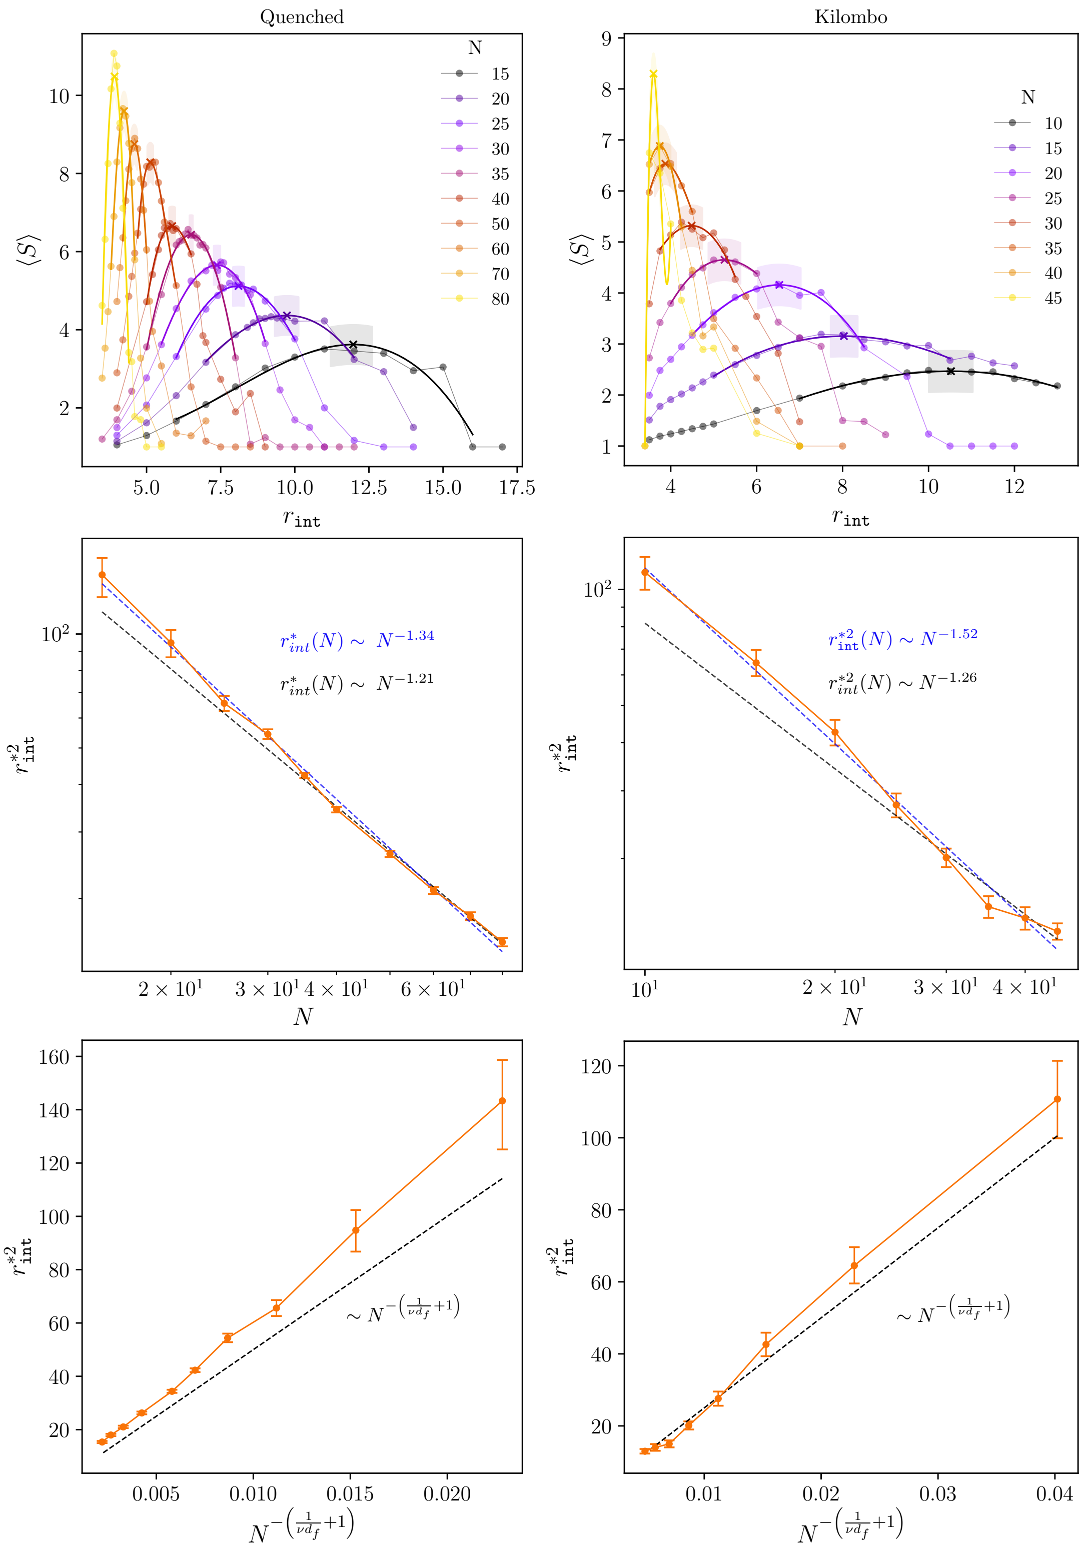


FIG. 5. Analysis performed to obtain the percolation value $r^*_{\mathtt{int}}$ and its finite-size dependence. It is shown both for quenched (left column) and kilombo configurations with $\Delta t = 800$ (right column). The **first row** depicts the mean cluster size, $\langle S \rangle$, as a function of the interaction radius. For each system size we identify the peak an fit a spline around it, in order to smoothly identify the percolation radius $r^*_{\mathtt{int}}$, along with an estimation of its error. The **second row** of figures shows the relation we obtain by fitting the squared critical value $r^{*2}_{\mathtt{int}}$ as a function of $N$. Possible fits are displayed, either considering the data error bars (black) or not considering them (blue). Finally, on the **bottom row** we show that our data fairly aligns with the 2D percolation theoretical prediction, specially at large $N$. The dashed line represents $r^{*2}_{\mathtt{int}} \sim N^{-(1+1/\nu d_f)}$, with $\nu = 4/3$ and $d_f = 91/48$.

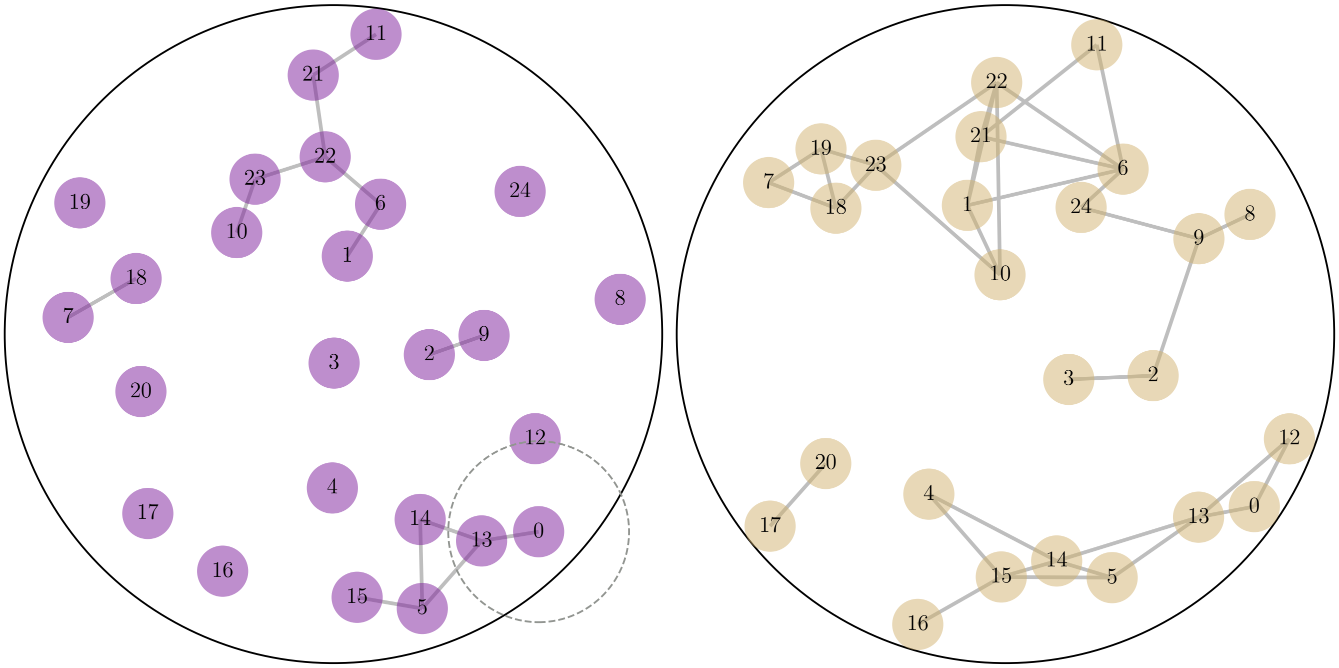


FIG. 6. Schematic representation of the kilombo simulations or kilobot experiments, indicating the contacts taking place within the swarm. **Left:** Snapshot of the positions and contacts taking place in the first compasses of a cycle of duration $\Delta t$. The connected agents are those whose separation $d_{i,j}$ is smaller than the interaction radius, $d_{i,j} < r_{\texttt{int}}$. The bots will perform a persistent random walk from these positions. **Right**: Snapshot of the positions of the kilobots at the end of the cycle. All the bots that have interacted during this period of time, i.e. those which momentary have satisfied the condition $d_{i,j} < r_{\texttt{int}}$, are now connected, in the *integrated* network of contacts corresponding to this cycle. Particular conditions are $N = 25$ and $r_{\texttt{int}} = 5.5$cm, while the arena radius is $R = 20.0$ cm. A video showing the movement and instantaneous contacts of the kilobots is also included as supplementary material.
